# Supplementary material for: Single-Stage 6D Object Pose Estimation
Source: arXiv:1911.08324 source file (2020-03-20)
Supplement: Supplementary file 1 [file 6_appendix.tex]

% !TEX root = ../top.tex
% !TEX spellcheck = en-US

\section{Appendix}
\label{sec:appendix}

\subsection{Derivation of quartic equations}
for a quartic function
$$f(x)=ax^4+bx^3+cx^2+dx+e,\quad a\neq0$$
\subsubsection{powers of complex number}
To computer the power of a complex number $z=a+ib$ (in our case, it is square root). We first convert the common rectangular form $z=a+ib$ to polar form $$z=r(\cos\theta + i\sin\theta),$$ where $a=r\cos\theta$ and $b=r\sin\theta$. The powers of complex number $z$ can be obtained by $$z^n=r^n[\cos(n\theta)+i\sin(n\theta)]$$.

\subsection{Vincent}
Hi Yinlin,

here is what I would do:

- Start with a random pose estimate: $pose_0 = (R_0, t_0)$

- Use a network F that predicts an update for the pose estimate. It could be done with the form:

$F( { Proj(pose_i, M_j) }_j, {m_j}_j ; Theta) = (DeltaR, Delta T)$

$pose_{i+1} = pose _i + F( { Proj(pose_i, M_j) }_j, {m_j}_j ; Theta)$   (1)

where $M_j$ are the 3D points (3d corners of the bounding box, for example), $m_j$ the predicted 2d projections for these 3D points (you currently get them with your voting scheme);
Proj() projects the 3D points M using the current pose estimate $pose_i$

You can iterate Eq (1) to get a better estimate.

- To train F(), you would optimise: 

$$\arg\min_{Theta}   \sum {examples   Dist}( pose_i + f( { proj(pose_i, M_j) }_j, {m_j}_j ; Theta), pose_{GT})$$

where $pose_{GT}$ is the ground truth pose = $(R_{GT}, t_{GT})$,

You need to define a distance Dist between 3D poses, you can use a simple weighted $sum (R - R_{GT}) + gamma (t - t_{GT})$, or better, you can look at :

https://arxiv.org/pdf/1612.04631.pdf

we can discuss further if it is not clear. 

Best,
Vincent
